# Supplementary material for: CARA: Exact Local Repair Queries for Cloud Consolidation
Source: arXiv:2607.29465 source file (2026-11-14)
Supplement: Supplementary file 1 [file supplement_results.tex]

% Result tables used by supplement.tex.
