# Supplementary material for: CARA: Exact Local Repair Queries for Cloud Consolidation
Source: arXiv:2607.29465 source file (2026-11-14)
Supplement: Supplementary file 2 [file supplement.tex]

\documentclass[letterpaper]{article}
\ifdefined\pdfsuppressptexinfo
  \pdfsuppressptexinfo=-1
\fi
\usepackage[preprint]{aaai2027}
\input{arxiv_layout.tex}
\usepackage[hyphens]{url}
\usepackage{graphicx}
\urlstyle{rm}

\usepackage{natbib}
\usepackage{amsmath}
\usepackage{amssymb}
\usepackage{booktabs}
\usepackage{array}
\usepackage{etoolbox}

% Always typeset table captions (and their labels) after the table body.
% This also applies to tables produced by macros loaded from the result files.
\makeatletter
\newif\ifcara@deferlabels
\newcommand{\cara@deferTableCaption}{%
  \cara@deferlabelsfalse
  \let\cara@originalcaption\caption
  \let\cara@originallabel\label
  \def\cara@savedcaptionmaterial{}%
  \long\def\cara@caption@plain##1{%
    \cara@deferlabelstrue
    \appto\cara@savedcaptionmaterial{\cara@originalcaption{##1}}%
  }%
  \long\def\cara@caption@short[##1]##2{%
    \cara@deferlabelstrue
    \appto\cara@savedcaptionmaterial{\cara@originalcaption[##1]{##2}}%
  }%
  \def\caption{\@ifnextchar[\cara@caption@short\cara@caption@plain}%
  \def\label##1{%
    \ifcara@deferlabels
      \appto\cara@savedcaptionmaterial{\cara@originallabel{##1}}%
    \else
      \cara@originallabel{##1}%
    \fi
  }%
}
\newcommand{\cara@flushTableCaption}{\cara@savedcaptionmaterial}
\AtBeginEnvironment{table}{\cara@deferTableCaption}
\AtEndEnvironment{table}{\cara@flushTableCaption}
\AtBeginEnvironment{table*}{\cara@deferTableCaption}
\AtEndEnvironment{table*}{\cara@flushTableCaption}
\makeatother

\pdfinfo{/TemplateVersion (2027.1)}
\frenchspacing
\setcounter{secnumdepth}{0}

\newcommand{\method}{\textsc{CARA}}
\newcommand{\strp}{\pi^{\mathrm{str}}}
\newcommand{\incp}{\pi^{\mathrm{I}}}
\newcommand{\candp}{\pi}

\DeclareMathOperator*{\argmax}{arg\,max}

% Result tables and narratives.
% Result tables used by supplement.tex.
\newcommand{\CARASuppPrimaryTable}{%
\begin{table*}[t]\centering\scriptsize\setlength{\tabcolsep}{2.5pt}
\caption{Complete registered incumbent-relative inference. Lower is better. Every endpoint requires a zero-margin one-sided mean-superiority bound and an exact sign-dominance test; the J row also includes the observed $-.005$ safeguard. Hosts are excluded because exact per-scene equality is a construction invariant.}
\label{tab:supp-primary}
\begin{tabular}{llrrrrrrlll}\toprule
Endpoint & Mode & Null & CARA & Frozen inc. & $\Delta$ & $U_{.95}$ & $p_t$ & $n_-/n_+/n_0$ & $p_s$ & Gate\\\midrule
$J$ & Superiority & 0 & 0.9323 & 0.9679 & -0.0357 & -0.0324 & $<.0001$ & 128/0/0 & $<.0001$ & Pass\\
$V$ & Superiority & 0 & 0.1506 & 0.1915 & -0.0409 & -0.0383 & $<.0001$ & 128/0/0 & $<.0001$ & Pass\\
$R$ & Superiority & 0 & 0.0132 & 0.0171 & -0.0040 & -0.0037 & $<.0001$ & 128/0/0 & $<.0001$ & Pass\\
$S$ & Superiority & 0 & 0.0471 & 0.0656 & -0.0185 & -0.0174 & $<.0001$ & 128/0/0 & $<.0001$ & Pass\\
Raw severity & Superiority & 0 & 0.000471 & 0.000656 & -0.000185 & -0.000174 & $<.0001$ & 128/0/0 & $<.0001$ & Pass\\
\bottomrule\end{tabular}\end{table*}%
}
\newcommand{\CARASuppJForestPlot}{%
\includegraphics[width=\columnwidth]{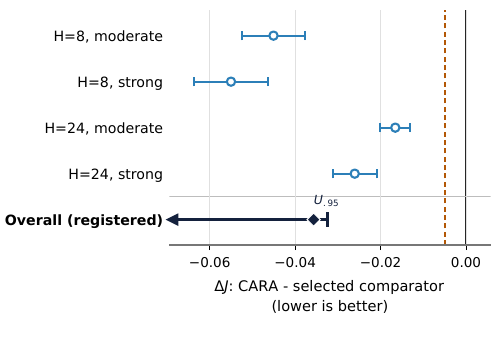}%
}
\newcommand{\CARASuppMechanismTable}{%
\begin{table*}[t]\centering\scriptsize\setlength{\tabcolsep}{3.2pt}
\caption{Descriptive paired \method{} minus \textsc{ProjBlind-2H} Evaluation contrast on all five endpoints. This is computed from the two terminal rows themselves, not by subtracting incumbent-relative summaries. The numerical all-five rule failed descriptively; exact host equality held. This contrast was not separately gatekept and is not a confirmatory mechanism claim.}
\label{tab:supp-projblind-descriptive}
\begin{tabular}{llrrrrll}\toprule
Endpoint & Mode & Null & $\Delta$ & $U_{.95}$ & $p_t$ & $p_s$ & Numerical rule\\\midrule
$J$ & Superiority & 0 & +0.0003 & +0.0007 & 0.9211 & 0.9637 & Fail\\
$V$ & Superiority & 0 & +0.0005 & +0.0009 & 0.9834 & 1.0000 & Fail\\
$R$ & Superiority & 0 & +0.0001 & +0.0001 & 0.9957 & 1.0000 & Fail\\
$S$ & Superiority & 0 & +0.0003 & +0.0004 & 0.9967 & 1.0000 & Fail\\
Raw severity & Superiority & 0 & +0.000003 & +0.000004 & 0.9967 & 1.0000 & Fail\\
\bottomrule\end{tabular}\end{table*}
\begin{table*}[t]\centering\small\setlength{\tabcolsep}{4pt}
\caption{Complete intention-to-treat Evaluation means for all six frozen policies. No policy or endpoint is selected for display.}
\label{tab:supp-six-policy}
\begin{tabular}{lrrrrrr}\toprule
Method & $J$ & $V$ & $R$ & $S$ & Raw & Hosts\\\midrule
\method{} & 0.9323 & 0.1506 & 0.0132 & 0.0471 & 0.000471 & 26.63\\
\textsc{Global96} & 0.9464 & 0.1612 & 0.0144 & 0.0530 & 0.000530 & 26.63\\
\textsc{ProjBlind-2H} & 0.9320 & 0.1500 & 0.0131 & 0.0468 & 0.000468 & 26.63\\
Frozen incumbent policy & 0.9679 & 0.1915 & 0.0171 & 0.0656 & 0.000656 & 26.63\\
\textsc{ILS} & 0.9651 & 0.1907 & 0.0170 & 0.0649 & 0.000649 & 26.63\\
\textsc{ALNS} & 0.9679 & 0.1915 & 0.0171 & 0.0656 & 0.000656 & 26.63\\
\bottomrule\end{tabular}\end{table*}
\begin{table*}[t]\centering\scriptsize\setlength{\tabcolsep}{2.7pt}
\caption{Complete stage flow over all 512 formal cells. A precommitted recovery procedure assigned the fixed reference action to all policies in 3 cell(s); 40 cell(s) used the preregistered structural-$H_0$ ITT zero rule. Both statuses remain visible. In available-incumbent cells the selected reference row is direct deployment and has no Search, raw-direction, Guard, or Certification operation; structural cells retain their generator terminal and reference fallback. Dashes denote inapplicability.}
\label{tab:supp-stage-flow}
\begin{tabular}{lrrrrrrrrr}\toprule
Method & Search & Raw pass & No alarm & Cert. & Release & Fallback & Cand./cell & Nodes & Bounds\\\midrule
\method{} & 469/512 & 469/512 & 469/512 & 445/469 & 445/512 & 67/512 & 14.66 & 32944186 & 28086939\\
\textsc{Global96} & 404/512 & 359/512 & 353/512 & 281/353 & 281/512 & 231/512 & 7.35 & 48864 & 6301\\
\textsc{ProjBlind-2H} & 468/512 & 468/512 & 468/512 & 448/468 & 448/512 & 64/512 & 14.62 & 32644608 & 114094\\
Frozen incumbent policy & 0/512 & 0/512 & 0/512 & -- & 0/512 & 40/512 & 0.00 & 17701735 & 862\\
\textsc{ILS} & 28/512 & 27/512 & 27/512 & 17/27 & 17/512 & 495/512 & 0.88 & 2623124 & 594109\\
\textsc{ALNS} & 0/512 & 0/512 & 0/512 & -- & 0/512 & 512/512 & 0.00 & 810300 & 356891\\
\bottomrule\end{tabular}\end{table*}%
}

% Public-trace result tables used by supplement.tex.
\newcommand{\CARATraceCoverageFunnel}{The complete coverage funnel is 20 Search attempts $\rightarrow$ 5 candidate-bearing episodes $\rightarrow$ 3 episodes entering the short screen $\rightarrow$ 0 releases. Specifically, 15 searches completed with no eligible block; all five candidate-bearing episodes were from Borg-d, two passed e-Guard but failed the raw-direction gate, and every $J/V/R/S$ screen component failed in each of the remaining 3 episodes. All 20 searches completed within the registered 500,000-node and 500,000-bound-evaluation caps; the largest recorded node count was 185,955. The rolling cases remain dependent sensitivity cases: within each trace their Evaluation windows are pairwise disjoint, but the 288-time-point histories at a 48-time-point stride overlap by 240 adjacent time points (144 common to all four histories), and the frozen cohorts share 43--48 of 48 items pairwise. No independent-replicate or provider-population inference is made.}
\newcommand{\CARASuppExternalNarrative}{\CARATraceCoverageFunnel{} Tables~\ref{tab:trace-primary} and~\ref{tab:trace-rolling} report every \method{} trace--origin outcome. Incumbent rows are omitted because all incumbent-relative differences are identically zero by construction.}
\newcommand{\CARASuppExternalTables}{%
\begin{table*}[t]\centering\scriptsize\setlength{\tabcolsep}{3.0pt}
\caption{Public-trace outcomes for one role-disjoint primary episode per trace. Lower is better. The incumbent source identifies the generator used by the frozen roster. All \method{} trace outcomes and endpoint differences are shown; the omitted incumbent rows are zero by construction. These named cases support no provider-population inference.}
\label{tab:trace-primary}
\begin{tabular}{r r l l r r r r r r}\toprule
Trace & Origin & Incumbent source & Terminal state & $\Delta J$ & $\Delta V$ & $\Delta R$ & $\Delta S$ & $\Delta$Raw & $\Delta H$\\\midrule
Azure & 528 & Verified evacuation & No candidate & +0.000 & +0.00000 & +0.00000 & +0.00000 & +0.00000 & +0\\
Borg-d & 528 & Verified evacuation & Guard veto & +0.000 & +0.00000 & +0.00000 & +0.00000 & +0.00000 & +0\\
Borg-e & 528 & Verified evacuation & No candidate & +0.000 & +0.00000 & +0.00000 & +0.00000 & +0.00000 & +0\\
Huawei & 528 & Verified evacuation & No candidate & +0.000 & +0.00000 & +0.00000 & +0.00000 & +0.00000 & +0\\
\bottomrule\end{tabular}\end{table*}
\begin{table*}[t]\centering\scriptsize\setlength{\tabcolsep}{3.0pt}
\caption{Public-trace outcomes for the four dependent rolling-history origins per trace. Lower is better. All \method{} trace--origin outcomes are retained; omitted incumbent rows are zero by construction. The rolling origins are sensitivity cases, not independent replications.}
\label{tab:trace-rolling}
\begin{tabular}{r r l l r r r r r r}\toprule
Trace & Origin & Incumbent source & Terminal state & $\Delta J$ & $\Delta V$ & $\Delta R$ & $\Delta S$ & $\Delta$Raw & $\Delta H$\\\midrule
Azure & 336 & Verified evacuation & No candidate & +0.000 & +0.00000 & +0.00000 & +0.00000 & +0.00000 & +0\\
Azure & 384 & \textsc{Global96} & No candidate & +0.000 & +0.00000 & +0.00000 & +0.00000 & +0.00000 & +0\\
Azure & 432 & Verified evacuation & No candidate & +0.000 & +0.00000 & +0.00000 & +0.00000 & +0.00000 & +0\\
Azure & 480 & \textsc{Global96} & No candidate & +0.000 & +0.00000 & +0.00000 & +0.00000 & +0.00000 & +0\\
Borg-d & 336 & Verified evacuation & Guard veto & +0.000 & +0.00000 & +0.00000 & +0.00000 & +0.00000 & +0\\
Borg-d & 384 & Verified evacuation & Screen failure & +0.000 & +0.00000 & +0.00000 & +0.00000 & +0.00000 & +0\\
Borg-d & 432 & Verified evacuation & Screen failure & +0.000 & +0.00000 & +0.00000 & +0.00000 & +0.00000 & +0\\
Borg-d & 480 & Verified evacuation & Screen failure & +0.000 & +0.00000 & +0.00000 & +0.00000 & +0.00000 & +0\\
Borg-e & 336 & Verified evacuation & No candidate & +0.000 & +0.00000 & +0.00000 & +0.00000 & +0.00000 & +0\\
Borg-e & 384 & Verified evacuation & No candidate & +0.000 & +0.00000 & +0.00000 & +0.00000 & +0.00000 & +0\\
Borg-e & 432 & Verified evacuation & No candidate & +0.000 & +0.00000 & +0.00000 & +0.00000 & +0.00000 & +0\\
Borg-e & 480 & Verified evacuation & No candidate & +0.000 & +0.00000 & +0.00000 & +0.00000 & +0.00000 & +0\\
Huawei & 336 & Verified evacuation & No candidate & +0.000 & +0.00000 & +0.00000 & +0.00000 & +0.00000 & +0\\
Huawei & 384 & Verified evacuation & No candidate & +0.000 & +0.00000 & +0.00000 & +0.00000 & +0.00000 & +0\\
Huawei & 432 & Verified evacuation & No candidate & +0.000 & +0.00000 & +0.00000 & +0.00000 & +0.00000 & +0\\
Huawei & 480 & Verified evacuation & No candidate & +0.000 & +0.00000 & +0.00000 & +0.00000 & +0.00000 & +0\\
\bottomrule\end{tabular}\end{table*}
}

% Shifted-Evaluation result-table macros used by supplement.tex.
\newcommand{\CARATerminalOODNarrative}{On fresh Evaluation banks under the prospectively frozen $0.35$ deployment shift, the already committed \method{} terminal action passed both the one-sided mean and exact non-tie sign components for all five endpoints across 128 synthetic environment clusters (512 repeated-context cells).  This is terminal-action robustness evidence only; it neither reruns nor validates the end-to-end OOD selection-and-release pipeline.}
\newcommand{\CARATerminalOODPrimaryRows}{%
$J$ & $0.9968$ & $0.9985$ & $-0.0017$ & $-0.0013$ & 99/11/18 & $<.0001$ & Pass\\
$V$ & $0.3877$ & $0.4166$ & $-0.0289$ & $-0.0261$ & 128/0/0 & $<.0001$ & Pass\\
$R$ & $0.0406$ & $0.0470$ & $-0.0063$ & $-0.0058$ & 128/0/0 & $<.0001$ & Pass\\
$S$ & $0.2211$ & $0.2714$ & $-0.0503$ & $-0.0461$ & 128/0/0 & $<.0001$ & Pass\\
Raw & $0.002224$ & $0.002734$ & $-0.0005$ & $-0.0005$ & 128/0/0 & $<.0001$ & Pass\\}
\newcommand{\CARATerminalOODPrimaryTable}{%
\begin{table*}[t]\centering\scriptsize\setlength{\tabcolsep}{3.2pt}
\caption{Prospectively frozen terminal-action stress test under the registered $0.35$ deployment shift (\method{} minus frozen incumbent; lower is better; 128 synthetic environment clusters and 512 repeated-context cells). Each primary endpoint uses component $\alpha=.01$; the joint screen passes only if every one-sided Student upper endpoint is below zero and every exact non-tie sign test passes. This is not an end-to-end OOD policy experiment.}
\label{tab:terminal-ood-primary}
\begin{tabular}{lrrrrrrl}\toprule
Endpoint & \method{} & Frozen inc. & $\Delta$ & $U_{.99}$ & $n_-/n_+/n_0$ & $p_s$ & Gate\\\midrule
\CARATerminalOODPrimaryRows
\bottomrule\end{tabular}\end{table*}%
}
\newcommand{\CARATerminalOODContextRows}{%
$H=8$, moderate & $-0.0025$ [$-0.0015$] & $-0.0229$ [$-0.0187$] & $-0.0051$ [$-0.0042$] & $-0.0455$ [$-0.0376$] & $-0.0005$ [$-0.0004$]\\
$H=8$, strong & $-0.0043$ [$-0.0025$] & $-0.0262$ [$-0.0212$] & $-0.0060$ [$-0.0049$] & $-0.0499$ [$-0.0408$] & $-0.0005$ [$-0.0004$]\\
$H=24$, moderate & $0$ [$0$] & $-0.0267$ [$-0.0213$] & $-0.0068$ [$-0.0057$] & $-0.0510$ [$-0.0428$] & $-0.0005$ [$-0.0004$]\\
$H=24$, strong & $-7.63{\times}10^{-5}$ [$6.76{\times}10^{-5}$] & $-0.0399$ [$-0.0322$] & $-0.0074$ [$-0.0062$] & $-0.0547$ [$-0.0454$] & $-0.0005$ [$-0.0005$]\\}
\newcommand{\CARATerminalOODContextTable}{%
\begin{table*}[t]\centering\scriptsize\setlength{\tabcolsep}{2.8pt}
\caption{Complete context diagnostics for the frozen terminal-action stress test. Entries are $\widehat\Delta\,[U]$ in one fixed 20-member Bonferroni family. These repeated-context rows cannot replace or rescue the synthetic-environment-averaged primary screen.}
\label{tab:terminal-ood-context}
\begin{tabular}{lrrrrr}\toprule
Context & $J$ & $V$ & $R$ & $S$ & Raw\\\midrule
\CARATerminalOODContextRows
\bottomrule\end{tabular}\end{table*}%
}

\title{Supplementary Material for \method{}:\\
Exact Local Repair and Fresh One-Action Certification}

\author{
    Xiyang Zhang\textsuperscript{\rm 1,\rm 2},
    Yuanhe Tian\textsuperscript{\rm 1}\corresponding,
    Hongzhi Wang\textsuperscript{\rm 2}
}

\affiliations{
    \textsuperscript{\rm 1}Zhongguancun Academy\\
    \textsuperscript{\rm 2}Harbin Institute of Technology\\
    s-zhangxiy24@bza.edu.cn,
    tianyuanhe@zgci.ac.cn,
    wangzh@hit.edu.cn
}

\begin{document}
\maketitle

\appendix

\section{Scope and Reading Guide}

This supplement provides proofs, experimental protocol, complete results, and
robustness checks.  Four
boundaries matter: (i) \method{} is exact only for its certificate order in the
bounded neighborhood; (ii) matched \textsc{ProjBlind-2H} has a separate prefix
that never feeds \method{}; (iii) fresh Certification controls conditional
false four-endpoint release, while raw/e-Guard are screens; and (iv) Evaluation
tests five terminal endpoints.  Neither exactness claim implies global
optimality, order superiority, or release.

\begin{table*}[t]
\centering
\scriptsize
\setlength{\tabcolsep}{3pt}
\begin{tabular}{>{\raggedright\arraybackslash}p{0.18\textwidth}
                >{\raggedright\arraybackslash}p{0.29\textwidth}
                >{\raggedright\arraybackslash}p{0.26\textwidth}
                >{\raggedright\arraybackslash}p{0.20\textwidth}}
\toprule
Claim & Assumptions & Validation evidence & Not implied\\
\midrule
Exact \method{} prefix; ideal matched prefix separately & Complete common action
inventory; nonnegative loads; resolved \method{} arithmetic; caps not hit;
ideal special-function evaluation for matched proposition & Per-order
exhaustive comparison; strict-only pruning; complete feasibility checks and
action deduplication & A pooled
union; global, cross-order, or Pareto optimality; all-input binary64
special-function exactness\\
Conditional false-improvement control & Fresh paired Certification bank;
fixed incumbent, action, and plans; conditional sign-dominance and independence
given the transcript and realized discordance set; one moment
path per continuous endpoint &
Prespecified one-use bank access, exact McNemar tail, exact integer products,
and no candidate retry &
Provider-shift robustness, raw-severity improvement, or high release rate\\
Held-out raw/Guard screens & Fixed routed action; disjoint Guard rows;
pre-row conditional bounded no-harm nulls for e-Guard & Exact raw Q53
direction, fixed mixtures, threshold 100 & Population raw inference;
false-veto control for the raw gate or conditional on its pass\\
Evaluation all-five claim & 128 i.i.d. draws from the registered synthetic
environment law; zero-margin mean superiority and tie-conditional sign
dominance on five endpoints & Complete
$128\times4\times512$ table and per-cell committed-target assignment recount &
Population inference from four public traces (three provider families) or
realized power from a design model\\
\bottomrule
\end{tabular}
\caption{Claims, assumptions, and boundaries.}
\label{tab:claim-map}
\end{table*}

Ordinary failure retains the $H_0-1$ incumbent.  If no frozen generator can
construct one, the precommitted structural $H_0$ action is assigned to both
policies as an exact-zero intention-to-treat state.  Family-integrity loss is
irrecoverable rather than silently mapped to that state; statistical
non-release in an available cell therefore preserves the existing host saving.

\section{Incumbent, Structural Scaffold, and Action Class}
\label{sec:registered-problem}

There are $N$ VMs, $T$ time coordinates, nonnegative scene loads
$x_{bit}\ge0$, and capacities $C_t>0$.  Fit estimates a factor--diagonal
covariance model and constructs a fully replayed structural placement
$\strp$ with $H_0$ hosts.  It defines feasibility and a fixed normalization,
but is not the ordinary statistical comparator.

Development-B contains ten independently seeded environments and four
contexts.  In each of its 40 cells, all five generators construct direct
$H_0-1$ actions using Fit and Build only.  A disjoint direct-Evaluation view
scores those fixed actions.  Lower-is-better within-cell midranks are computed
for $J,V,R,S$, and raw.  The frozen rule first maximizes the number of eligible
cells and then applies full leximin to the increasingly sorted $40\times5$ rank
vector; fixed method order breaks a complete tie.  This selects the first
generator and the remaining fallback order.

In a formal cell, generators are tried in frozen order on the committed
Fit/Search/Plan view.  The first nonempty output is reranked by the exact
four-endpoint projected-certificate key; the canonical physical action identity
breaks ties.

\newpage
Its first action is the certificate-reranked frozen-generator incumbent
$\incp$.

The action and selection rule are committed before any Screen, Certification,
or Evaluation outcomes exist.  If all registered generators are empty, the
cell retains the structural $H_0$ reference as an exact-zero intention-to-treat
state; no post-outcome replacement is allowed.

An outcome-frozen seed pool supplies verified $H_0-1$ placements.  For seed
$s$ and an unordered pair of its nonempty hosts $(h_1,h_2)$, let
$U_{s,h_1,h_2}$ be their item union.  A block is eligible when
$2\le|U_{s,h_1,h_2}|\le m$.  All other hosts remain fixed, while the block
contains every bipartition $(A,U\setminus A)$ with both parts nonempty.  The
smallest mutable VM is fixed to the first replacement host, and replacement
hosts are canonically relabeled, removing the two-way label symmetry.

A complete leaf is replayed independently for item coverage, nonempty hosts,
cardinality, capacity, covariance feasibility, and exactly $H_0-1$ active
hosts.  A canonical action encoding deduplicates placements while preserving
origins,
and the unchanged incumbent is removed.  The neighborhood is narrower than
global packing and broader than one-donor evacuation: items may move both
ways.  Exact packing, ranked solutions, and multiobjective search remain prior art
\cite{murty1968ranking,coffman1996binpacking,scholl1997bison,
przybylski2017multiobjective}; the new object is the incumbent-relative
admissible bound in the mixed certificate lattice.

\subsection{Fixed-normalizer burdens}

For placement $\pi$ and scene $b$, define
\[
q_{bht}(\pi)=
 \left[\sum_{i:\pi(i)=h}x_{bit}-C_t\right]_+/C_t.
\]
Let $D_b(\pi)$ count hosts with an overload beyond the registered tolerance,
$L_b(\pi)$ count violating host--time pairs, and
$E_b(\pi)=\sum_{h,t}q_{bht}(\pi)$.  The bounded burdens are
\begin{align}
J_b(\pi)&=\mathbf1\{D_b(\pi)>0\},\qquad
V_b(\pi)=D_b(\pi)/H_0,\nonumber\\
R_b(\pi)&=L_b(\pi)/(H_0T),\nonumber\\
S_b(\pi)&=\min\{E_b(\pi)/(\kappa H_0T),1\}.
\label{eq:supp-burdens}
\end{align}
Raw severity $u_b(\pi)=E_b(\pi)/(H_0T)$ is stored separately.  Guard uses
$\rho_b(\pi)=u_b/(u_b+\kappa)$ because betting factors require bounded
increments; its mean does not identify the mean of $u_b$.  Both $\incp$ and
$\candp$ use the same $H_0$ denominator and exactly $H_0-1$ hosts, so the
comparison changes neither exposure nor structural host count.

\section{Exact Incumbent-Relative Certificate Search}
\label{sec:exact-search-proof}

Write $n_B$ for Search/Plan size, $n_C$ for Certification size, and
$r=n_C/n_B\in\mathbb N$; here $n_B=256$, $n_C=8192$, and $r=32$.  For $J$,
$A$ counts candidate-only harmful Build discordances and $B$ counts
incumbent-only harmful discordances.  Define
\begin{align}
p_J(A,B)&=\Pr\{\operatorname{Bin}(r(A+B),1/2)\le rA\},\nonumber\\
\theta_J(A,B)&=\log(1/20)-\log p_J(A,B).
\label{eq:supp-j-margin}
\end{align}
For $e\in\{V,R,S\}$, let $M=2^{53}$ and, for stored binary64 $z\in[0,1]$,
define the closed-midpoint count
\begin{equation}
\begin{aligned}
C_{53}(z)
&=\left|\left\{k\in\{0,\ldots,M-1\}:\frac{k+1/2}{M}\le z\right\}\right|\\
&=\lfloor Mz+1/2\rfloor.
\end{aligned}
\label{eq:supp-q53-count}
\end{equation}
Thus $C_{53}(z)\in\{0,\ldots,M\}$ and
$|C_{53}(z)/M-z|\le1/(2M)$.  Put
\begin{align}
d_{ei}&=C_{53}(e_i(\incp))-C_{53}(e_i(\candp)),\nonumber\\
X_{ei}&=(d_{ei}-1)/(M+1).
\label{eq:supp-q53}
\end{align}
$d_{ei}\in[-M,M]$ and
$X_{ei}\in[-1,(M-1)/(M+1)]$, so all registered betting factors are strictly
positive.
The Build fitter exhausts $j\in\{0,\ldots,255\}$ and computes
\begin{align}
g_e(j)&=\sum_{i=1}^{n_B}\log\!\left(1+\frac{j}{256}X_{ei}\right),\nonumber\\
b_e(j)&=\operatorname{round}_{\rm even}\{2^{40}g_e(j)\}.
\label{eq:build-plan-fit}
\end{align}
It maximizes $(b_e(j),g_e(j),-j)$ lexicographically under the specified
binary64 \texttt{log1p}/\texttt{fsum} rule and fixes
$\lambda_e=j_e/256$.  Search then encloses
\begin{equation}
\theta_e=r\sum_{i=1}^{n_B}\log(1+\lambda_eX_{ei})-\log20
\label{eq:supp-cont-margin}
\end{equation}
from the exact rational factors.  These target-size quantities are ranking
margins, not evidence from the future Certification bank.

\paragraph{Certificate-form alignment.}
Fix an action and $\lambda_e$ before both Build and Certification panels, and
suppose their rows are i.i.d. from the same conditional law.  For
$Y_e=\log(1+\lambda_eX_e)$, $r n_B=n_C$ gives
$\mathbb E[r\sum_{i=1}^{n_B}Y_{ei}-\log20]=n_C\mathbb E Y_e-\log20$.
Moreover $Y_e\in[-\log256,\log2]$.  Applying Hoeffding to the fresh sum
$\log W_e=\sum_{i=1}^{n_C}Y_{ei}$ proves the bound in the main text whenever
$\mathbb E Y_e>\log20/n_C$.  The fixed-pair premise is essential: adaptive
Build selection prevents interpreting the observed projection as an unbiased
post-selection estimate or confidence bound.

\subsection{Lattice key and traversal}

Let $\eta=2^{-40}$.  Directed intervals for each $\theta_e$ are refined until
their lower and upper endpoints have the same $\eta$-floor.  The corresponding
integer $s_e=\lfloor\theta_e/\eta\rfloor$ is then unique.  A leaf key sorts its
four labeled scores increasingly and compares the vectors lexicographically;
only a complete evidence tie reaches the canonical physical assignment.

\noindent\textbf{Proposition 1 (conjunctive lattice margin).}
For $\mathcal C=\{s\in\mathbb Z^4:s_e\ge0\ \forall e\}$,
\[
 \sup\{\delta\in\mathbb Z:s-\delta\mathbf1\in\mathcal C\}=\min_es_e.
\]
Full leximin first maximizes this signed uniform-shift margin and, conditional
on a tie, recursively maximizes every remaining bottleneck.

\noindent\emph{Proof.}
Membership after a shift is equivalent to $\delta\le s_e$ for every
coordinate.  The largest feasible shift is therefore the minimum coordinate.
Sorting exposes that minimum first; fixing equal leading coordinates and
repeating proves the recursive claim. \hfill$\square$

Search iterates the canonical seed--block inventory, applies the symmetry
break, and recursively assigns the remaining mutable VMs.  At a complete node
it replays all physical constraints, fits the three plans, resolves the
lattice key, deduplicates the action, rejects $\incp$, and updates an ordered
top-$P$ set.  A partial node first applies the hereditary structural check
below; otherwise it computes the evidence bound.  Once $P$ distinct actions exist,
evidence pruning requires the optimistic sorted vector to be strictly below
the current $P$th vector.  An arithmetic ceiling, node cap, or bound cap
exposes no partial prefix and returns the incumbent path.

\subsection{Admissibility of the partial bound}

\noindent\textbf{Lemma (monotone structural pruning).}
If a partial replacement host exceeds the physical cardinality cap or its
fitted mean load exceeds capacity (including the registered tolerance) at any
time, no descendant is valid.

\noindent\emph{Proof.}
Every descendant only adds VMs to that host.  Cardinality and every fitted
mean-load coordinate are therefore nondecreasing because fitted item means
are nonnegative.  Covariance is not partially pruned; it is replayed at each
complete leaf. \hfill$\square$

Let $F_n(k)=\Pr\{\operatorname{Bin}(n,1/2)\le k\}$.  Conditioning on the last
Bernoulli trial gives
\begin{align}
F_{n+1}(k+1)
  &=\tfrac12F_n(k+1)+\tfrac12F_n(k)\notag\\
  &\ge F_n(k),
\label{eq:rec1}\\
F_n(k)
  &=\tfrac12F_{n-1}(k)+\tfrac12F_{n-1}(k-1)\notag\\
  &\le F_{n-1}(k).
\label{eq:rec2}
\end{align}

\noindent\textbf{Lemma 1 (projected McNemar monotonicity).}
Turning one partial candidate $J$ value from zero to one cannot increase
$\theta_J$ for any positive integer projection ratio $r$.

\noindent\emph{Proof.}
If the incumbent bit is zero, $(A,B)$ becomes $(A+1,B)$; repeated use of
Eq.~\eqref{eq:rec1} shows that the projected lower-tail probability cannot
decrease.  If the incumbent bit is one, $(A,B)$ becomes $(A,B-1)$; repeated
use of Eq.~\eqref{eq:rec2} gives the same conclusion.  Since $-\log p$ is
nonincreasing in $p$, the margin cannot improve. \hfill$\square$

Omitting unassigned VMs produces componentwise lower candidate burdens because
loads are nonnegative.  Adding an item can only decrease each
incumbent-minus-candidate midpoint difference.  For fixed nonnegative
$\lambda$, $\log(1+\lambda X)$ is increasing in $X$.

\noindent\textbf{Lemma 2 (plan-independent continuous bound).}
At a partial node $v$, let $X_i(v)$ be the corrected difference obtained by
omitting unassigned VMs.  For every descendant action $a$, its fitted
$0\le\lambda_a\le255/256$ satisfies
\begin{equation}
\theta_e(a)
\le r\frac{255}{256}\sum_i\max\{X_i(v),0\}-\log20
=:\overline\theta_e(v),
\label{eq:continuous-bound}
\end{equation}
The outward upward lattice rounding of $\overline\theta_e(v)$ bounds every
descendant score, independently of the descendant's fitted plan.

\noindent\emph{Proof.}
Partial differences satisfy $X_i(v)\ge X_i(a)$.  Since
$X_i(a)\ge-1$ and $\lambda_a<1$, each factor is positive and
$\log(1+\lambda_aX_i(a))\le\lambda_aX_i(a)
\le(255/256)\max\{X_i(v),0\}$.  Summation, multiplication by $r$, subtraction
of $\log20$, and upward rounding preserve the inequality.  For $S$, the
implementation uses zero partial severity, a looser bound that remains valid
by nonnegativity. \hfill$\square$

\noindent\textbf{Lemma 3 (sorting preserves optimism).}
If $u_e\ge v_e$ for every labeled coordinate, then the $k$th increasing order
statistic of $u$ is at least that of $v$ for every $k$.

\noindent\emph{Proof.}
Otherwise at least $k$ components of $u$ would lie below the $k$th order
statistic of $v$.  Their labeled counterparts in $v$ are no larger, which
contradicts the definition of that order statistic. \hfill$\square$

\noindent\textbf{Theorem 1 (incumbent-anchored exact neighborhood top-$P$).}
Let $\mathcal A(\incp)$ be all distinct, replay-valid actions other than
$\incp$ in the registered seed--block neighborhood.  If the typed inputs
validate, all required replays and arithmetic intervals resolve, and neither
work cap is reached, strict-only branch-and-bound returns the first
$\min\{P,|\mathcal A(\incp)|\}$ actions under the decreasing full-leximin
lattice key followed by increasing canonical physical assignment.

\noindent\emph{Proof.}
The symmetry-broken tree represents one copy of every nonempty bipartition.
The structural-pruning lemma discards no valid completion, and Lemmas 1--3
make the partial sorted key optimistic for every descendant.  A subtree
pruned on a strict evidence loss cannot contain an action that enters the
retained prefix.  Equality is never pruned before its physical tie row is
known.  Complete replay removes exactly invalid leaves; global canonical
encoding merges only identical assignments; explicit anchor rejection removes
only $\incp$.  Induction over the deterministic traversal therefore yields
the same ordered distinct-action prefix as exhaustive enumeration.
\hfill$\square$

With $S$ seeds and at most $H$ hosts per seed, there are at most
$S\binom H2$ blocks and $O(2^m)$ structural nodes per eligible block.  Under
the fixed precision schedule and work caps, replay, plan fitting, interval
resolution, and top-$P$ maintenance have finite cost per node.  Given the
seeds, the structural node count is fixed-parameter tractable in $m$; seed
generation lies outside this bound.  No claim is made for unrestricted global
bin packing or unit-cost transcendental arithmetic.

Exact recovery in Theorem~1 means fidelity to the registered
certificate objective.  It does not assert that this objective is statistically
or operationally superior to another proposal order.

\section{Ideal-Arithmetic Prefix for the Matched Directional Comparator}
\label{sec:directional-prefix-proof}

\textsc{ProjBlind-2H} is a separate matched comparator.  It uses the same
committed seed authority, eligible
two-host blocks, symmetry break, complete physical replay, incumbent exclusion,
and canonical physical action identity as Section~\ref{sec:exact-search-proof}.
It differs only in its Build ranking, and its prefix never enters \method{}
Cover, Route, or Certification.  Let $x_{eb}(\pi)$ be action $\pi$'s
bounded burden for $e\in\{J,V,R,S\}$ on Build scene $b$, and let
$x_{eb}(\strp)$ be the fixed structural-reference burden.  Define the
candidate-only and reference-only directional masses
\begin{align}
 A_e(\pi)&=\sum_b[x_{eb}(\pi)-x_{eb}(\strp)]_+,\nonumber\\
 B_e(\pi)&=\sum_b[x_{eb}(\strp)-x_{eb}(\pi)]_+.
\label{eq:directional-masses}
\end{align}
For $J$ these are integer discordance counts; for $V,R,S$ they are nonnegative
fractional masses.  They are deterministic Build ranking surrogates, not
Certification $p$-values.

For nonnegative $A,B$, write
\begin{align}
 g(A,B)&=\log(1/20)-\log I_{1/2}(B,A+1),\nonumber\\
 q(A,B)&=F_{\lceil A\rceil+\lfloor B\rfloor}(\lceil A\rceil),\qquad
 d(A,B)=B-A,
\label{eq:directional-rb-components}
\end{align}
where $I$ is the regularized incomplete beta function, its registered $B=0$
limit is one, and $F_n(k)=\Pr\{\operatorname{Bin}(n,1/2)\le k\}$.  On integer
masses, the fractional tail in $g$ equals the one-sided conditional McNemar
tail; $q$ is its conservative exact-grid anchor for fractional masses.  Put
$g_e(\pi)=g(A_e(\pi),B_e(\pi))$, and analogously define $q_e(\pi)$ and
$d_e(\pi)$.  The directional key compares, in order,
\begin{equation}
 \left(
  \operatorname{sort}_{\uparrow}\{g_e(\pi)\}_e,
  \operatorname{sort}_{\downarrow}\{q_e(\pi)\}_e,
  \operatorname{sort}_{\uparrow}\{d_e(\pi)\}_e
 \right).
\label{eq:directional-rb-key}
\end{equation}
The first and third rows are lexicographically maximized, while the second is
lexicographically minimized.  The registered unary $2^{-40}$ comparison
buckets are applied to the finite binary64 entries of the first and third
rows.  Comparator equality is broken by increasing canonical physical
assignment.  This defines a deterministic total order on distinct actions.

\subsection{Node optimism and exactness}

At depth $d$, unassigned block VMs are omitted.  By nonnegative loads, every
complete descendant $z$ has
$x_{eb}^{(d)}\le x_{eb}^{(z)}$ for every labeled endpoint and scene.  Relative
to the fixed $x_{eb}(\strp)$, positive-part monotonicity gives
\begin{equation}
 A_e^{(d)}\le A_e^{(z)},\qquad B_e^{(d)}\ge B_e^{(z)}.
\label{eq:directional-node-mass-order}
\end{equation}
The implemented node bound does not rely on ideal real arithmetic.  Let $N$
be the Build panel size, let $u=2^{-53}$ be binary64 unit roundoff, and define
the registered absolute radius
\begin{equation}
 \varepsilon_N=\min\{N,\,8(N+1)^2u\}.
\label{eq:directional-float-radius}
\end{equation}
For $J$, masses are exact counts.  For $V$ and $R$, the node reduces exact
integer directional numerators, divides once, subtracts $\varepsilon_N$ from
the harmful-mass center and adds it to the beneficial-mass center, clips to
$[0,N]$, and takes one outward \texttt{nextafter} step.  For $S$, it uses the
universal candidate lower burden zero, hence harmful mass zero, and adds the
same radius plus an outward step to the fixed-reference sum.

To justify the radius, every replayed burden and positive-part term lies in
$[0,1]$.  Applying the standard binary64 model to the two divisions,
subtraction, positive part, and final faithfully rounded sum gives absolute
forward error at most $8(N+1)^2u$ whenever $8(N+1)u<1$; the registered
$N=256$ is in this regime.  If the expression is not informative, clipping
$\varepsilon_N$ to $N$ returns the whole possible mass range.  Thus the
additional outward step encloses the corresponding complete binary64 replay in
all cases.

\noindent\textbf{Lemma (ideal directional RB node optimism).}
With the incomplete-beta component evaluated in ideal real arithmetic, the
conservative directional key at any visited node is no worse than the exact key
of every physically feasible complete descendant.

\noindent\emph{Proof.}
For positive shapes, write a beta variate as $Y/(Y+Z)$ with independent gamma
variables of shapes $B$ and $A+1$.  Increasing $B$ couples by adding an
independent gamma increment to $Y$ and shifts this ratio upward; increasing $A$
adds an independent gamma increment to $Z$ and shifts it downward.  Hence
decreasing $A$ or increasing $B$
cannot increase the incomplete-beta lower tail at $1/2$; the registered
zero-shape limit has the same direction.  Equation
\eqref{eq:directional-node-mass-order} therefore makes $g$ optimistic.  The
same mass changes cannot increase the exact-grid McNemar tail $q$, by the
binomial recurrences in Eqs.~\eqref{eq:rec1}--\eqref{eq:rec2}, and cannot
decrease $B-A$.  Outward mass envelopes preserve these directions against
complete binary64 replay.  Labeled componentwise dominance preserves all three
sorted order-statistic rows, and the unary comparison buckets are monotone.
Hence the complete node key is no worse than every descendant key.
\hfill$\square$

\noindent\textbf{Proposition 2 (matched directional ideal prefix).}
Let $\mathcal A(\incp)$ be the registered bounded two-host family in
Theorem~1.  If typed inputs validate, all required physical replays finish, the
registered work cap is not reached, and $I_{1/2}$ is evaluated exactly, the
ideal directional search returns the first
$\min\{P,|\mathcal A(\incp)|\}$ distinct actions under
Eq.~\eqref{eq:directional-rb-key} and the canonical physical tie row.

\noindent\emph{Proof.}
For every verified seed, every unordered eligible host pair is visited.  Fixing
the smallest mutable VM to the first replacement host enumerates each unordered
nonempty bipartition once within a block.  Hereditary cardinality and fitted
mean-capacity failures remove no feasible completion; covariance is checked
only at leaves.  By the ideal directional node-optimism lemma, a node whose key is
strictly worse than the current $P$th complete action cannot enter the retained
prefix.  Comparator equality is not pruned because the descendant's canonical
physical tie row is unknown.
Every surviving leaf receives complete feasibility and endpoint replay;
incumbent exclusion precedes top-$P$ insertion; canonical assignment merges
only the same physical action across seeds and blocks.  Sorted insertion and
truncation therefore maintain the same distinct-action prefix as exhaustive
enumeration throughout the deterministic traversal. \hfill$\square$

If a work cap is reached or a required replay or arithmetic operation does not
resolve, the comparator discards its partial retained list.  The implemented
comparator evaluates the incomplete beta function in binary64; exhaustive
small-instance parity checks its returned prefix, but we do not claim that the
library evaluation preserves every ideal $2^{-40}$ bucket on all possible
inputs.  Proposition~2 is therefore an ideal-order guarantee, not an all-input
executable special-function theorem.  It neither ranks that order above the
certificate objective nor changes \method{}'s one-fixed-action Certification
theorem.

\section{Arithmetic Contract and Q53 Transfer}
\label{sec:arithmetic}

Binary64 logs are used only in the Build plan-selection rule.  Once $j$ is
fixed, each continuous factor is the positive rational
\begin{equation}
\frac{256(M+1)+j(d_i-1)}{256(M+1)}.
\label{eq:integer-factor}
\end{equation}
Equal factors are grouped and powered before multiplication.  Certification
compares exact integer numerator $N$ and denominator $D$ through the inclusive
inequality $N\ge20D$.  Search evaluates logarithms under a fixed
precision-doubling schedule with outward rounding.  Refinement stops only when
both bounds occupy one lattice cell; crossing a boundary at the ceiling raises
a typed unresolved result.  The binary component uses exact binomial
recurrences and rational bounds.  Independent tests cover zero, adverse,
favorable, threshold-adjacent, and near-lattice inputs.

\noindent\textbf{Lemma 4 (Q53 correction transfers the mean null).}
For stored $a,b\in[0,1]$, let $d=C_{53}(b)-C_{53}(a)$.  Then
\begin{equation}
\frac{d-1}{M+1}\le\frac{M(b-a)}{M+1}.
\label{eq:q53-transfer}
\end{equation}
Thus, for any sigma-field $\mathcal K$,
$\mathbb E[b-a\mid\mathcal K]\le0$ implies
$\mathbb E[(d-1)/(M+1)\mid\mathcal K]\le0$.

\noindent\emph{Proof.}
Under the executable closed-midpoint convention,
$Mz-1/2\le C_{53}(z)\le Mz+1/2$.  Subtracting the lower bound for $C_{53}(a)$
from the upper bound for $C_{53}(b)$ yields $d\le M(b-a)+1$.
Conditional expectation preserves the resulting inequality. \hfill$\square$

\section{Conditional Certification Guarantee}
\label{sec:certification-proof}

Let $\Theta$ denote fixed environment parameters and let $\mathcal T_-$ be the
complete transcript through e-Guard: the structural scaffold, incumbent,
routed action, three fitted plans, all earlier outcomes and decisions, and the
endpoint definitions.  It excludes the Certification innovations and all
endpoint values determined by them.  Put
$\mathcal H_-=\sigma(\Theta,\mathcal T_-)$.  Prespecified Certification row
labels may occur in $\mathcal T_-$ only as ancillary indices: conditional on
$\Theta$, fresh innovations follow the registered law independently of the
upstream transcript.  In particular, the statistical argument does not
condition on a latent random-state variable that determines those innovations;
the audit record checks this separation but is not itself an independence
assumption.  The
routed action and each Build-selected
$\lambda_e\in[0,255/256]$ are $\mathcal H_-$-measurable.

For $J$, condition further on the realized discordance set $\mathcal D$.
Assume the discordant signs are independent given
$(\mathcal H_-,\mathcal D)$; under $H_J$, sign $i$ is candidate-only harmful
with conditional probability $p_i\ge1/2$.  Their sum is therefore a
Poisson--binomial variable that stochastically dominates
$\operatorname{Bin}(|\mathcal D|,1/2)$, making the fair-binomial lower tail
super-uniform.

For each $e\in\{V,R,S\}$, validity may be established under either registered
null path:
\begin{enumerate}
\item $H_e^{\rm seq}$ (\emph{sequential mean}):
$\mathbb E[X_{ei}\mid\mathcal H_-,X_{e,<i}]\le0$ for every row.
\item $H_e^{\rm ind}$ (\emph{independent average mean}): the rows are independent given
$\mathcal H_-$ and
$n_C^{-1}\sum_i\mathbb E[X_{ei}\mid\mathcal H_-]\le0$.
\end{enumerate}
Below, $H_e$ denotes the applicable registered path.
The second permits heterogeneous row means but not serial dependence; the first
permits history-adaptive laws but not later negative means compensating for a
positive conditional mean.  Sufficient conditions in the original burden
scale are, respectively,
$\mathbb E[e_i(\incp)-e_i(\candp)\mid
\mathcal H_-,X_{e,<i}]\le0$ for every $i$, or conditionally independent paired
rows with
$n_C^{-1}\sum_i\mathbb E[e_i(\incp)-e_i(\candp)\mid\mathcal H_-]\le0$.
Lemma~4 transfers these inequalities to $X_{ei}$; conditional independence is
inherited by the deterministic Q53 transforms.

\noindent\textbf{Lemma 5 (continuous component level).}
Under either path,
\[
\Pr\left\{\prod_{i=1}^{n_C}(1+\lambda_eX_{ei})\ge20
 \mid\mathcal H_-\right\}\le.05.
\]

\noindent\emph{Proof.}
Under the sequential path the product is a nonnegative supermartingale with
conditional expectation at most one.  Under the independent path, writing
$\mu_i=\mathbb E[X_{ei}\mid\mathcal H_-]$, factorization and AM--GM give
\begin{align*}
\mathbb E[W_{n_C}\mid\mathcal H_-]
&=\prod_i(1+\lambda_e\mu_i)\\
&\le\left(1+\lambda_en_C^{-1}\sum_i\mu_i\right)^{n_C}\le1.
\end{align*}
All random factors and all AM--GM terms are positive: $X_{ei}\ge-1$ and
$\mu_i\ge-1$ give $1+\lambda_eX_{ei}\ge1/256$ and
$1+\lambda_e\mu_i\ge1/256$.  Markov's inequality completes either path.
\hfill$\square$

\noindent\textbf{Theorem 2 (conditional false-improvement release).}
If at least one of $H_J,H_V,H_R,H_S$ is true, the probability that the exact
McNemar component and all three fixed-wealth components pass is at most $.05$,
conditional on $\mathcal H_-$.

\noindent\emph{Proof.}
Conditional on $(\mathcal H_-,\mathcal D)$, couple each independent
$\operatorname{Bernoulli}(p_i)$ sign with a fair Bernoulli by common uniforms.
The former sum is no smaller almost surely, so the fair-binomial lower-tail
test is conservative after averaging over $\mathcal D$.  The binary component
is therefore level $.05$ conditional on $\mathcal H_-$; Lemma 5
gives the same level for each continuous component.  Under the
intersection--union null, joint release is contained in at least one true-null
rejection event.  Its conditional probability is therefore at most $.05$;
no Bonferroni split is needed. \hfill$\square$

This is a terminal-product result, not an anytime claim
\cite{shafer2011martingales,ramdas2023gametheoretic}.  It applies to one action
fixed before its bank.  It
does not cover raw severity, cross-policy familywise error, population shift,
or the probability that Search finds an action worth releasing.

\section{Held-Out Choice, Direction Gate, and e-Guard}
\label{sec:staging}

Build and Screen are split by outcome-free identities.  Search/Plan generates
and scores actions.  Cover receives only the exact top-$P$ prefix and replays
it on four fixed folds.  For a held-out panel $G$, it recomputes the projected
$J$ margin and the three fixed-plan margins without refitting.  If $s_{afe}$
is action $a$'s endpoint lattice score on fold $f$, exact midranks first map
each endpoint among actions to $r_{afe}\in[0,1]$.  Put
$b_{af}=\min_er_{afe}$ and midrank these bottlenecks again to obtain
$q_{af}$.  Cover exhausts
\begin{equation}
\widehat S\in\argmax_{\emptyset\ne S\subseteq[P],\ |S|\le K}
\frac14\sum_{f=1}^{4}\max_{a\in S}q_{af},
\quad K=\min\{4,P\}.
\label{eq:supp-exact-cover}
\end{equation}
For $P\le16$, at most $\sum_{k=1}^4\binom{16}{k}=2{,}516$ subsets are
examined.  Equal values prefer the smaller set, then Search order and the canonical
physical action identity.  Route replays this portfolio on a disjoint Screen
half and chooses one
action by full leximin of endpoint ordinals centered at the zero certificate
boundary.  It cannot generate a new action or refit a plan.

The complementary Screen half goes only to the routed winner.  For any finite
nonnegative binary64 raw severity, define the unbounded integer count
\[
C^{\rm raw}_{53}(u)=\lfloor2^{53}u+1/2\rfloor.
\]
The raw-direction gate requires
\begin{equation}
 \sum_{i\in G}\{C^{\rm raw}_{53}(u_i(\incp))
 -C^{\rm raw}_{53}(u_i(\candp))-1\}\ge0.
\label{eq:supp-raw-direction}
\end{equation}
Because
$C^{\rm raw}_{53}(b)-C^{\rm raw}_{53}(a)-1\le2^{53}(b-a)$,
passing implies a nonpositive candidate-minus-incumbent raw mean on these
held-out rows.  The count is evaluated with unbounded integer arithmetic, so the gate does
not clip large finite raw values.  This is an observed-sample direction
check only; it supplies neither a population tail bound nor a raw-severity
safety certificate.

The raw gate and e-Guard use this same once-opened row batch; the former is not
a data split for the latter.  Before any outcome in $G$ is opened, let
$\mathcal T_G$ contain the fixed environment parameters, routed action,
incumbent, transforms, row identities and order, but neither a $G$-row outcome
nor PRNG state determining one, and put
$\mathcal F_G=\sigma(\mathcal T_G)$.  For e-Guard, let $M=2^{53}$ and use the
same closed-midpoint map
$C_M(z)=|\{k\in\{0,\ldots,M-1\}:(k+1/2)/M\le z\}|
=\lfloor Mz+1/2\rfloor\in\{0,\ldots,M\}$.
Let $\rho=\psi_\kappa(u)$ and $\mathcal E_G=\{J,V,R,S,\rho\}$.  Define
candidate-minus-incumbent increments
\begin{align}
Z_{iJ}&=J_i(\candp)-J_i(\incp),\nonumber\\
h_{ie}&=C_M(e_i(\candp))-C_M(e_i(\incp)),\nonumber\\
Z_{ie}&=(h_{ie}-1)/(M+1),\qquad e\in\{V,R,S,\rho\}.
\label{eq:supp-eguard-transform}
\end{align}
Here $h_{ie}\in[-M,M]$ and
$Z_{ie}\in[-1,(M-1)/(M+1)]$.
The registered fixed mixture is
\begin{equation}
G_e=\frac1{255}\sum_{j=1}^{255}\prod_{i\in G}
\left(1+\frac{j}{256}Z_{ie}\right).
\label{eq:supp-eguard-mixture}
\end{equation}
Guard vetoes iff some $G_e\ge100$; equality vetoes.  Products and the mixture
comparison are evaluated with exact integers.  Readiness and signed gains are
reported only as diagnostics.  No alarm forwards the same winner; it neither
certifies no harm nor unlocks another portfolio action.

\noindent\textbf{Proposition 3 (e-Guard false-veto control).}
Condition on $\mathcal F_G$.  Suppose all five transformed
candidate-minus-incumbent no-harm nulls hold conditionally.  For each endpoint
assume either
$\mathbb E[Z_{ie}\mid\mathcal F_G,Z_{<i,e}]\le0$ for every row, or conditional
independence given $\mathcal F_G$ with
$|G|^{-1}\sum_{i\in G}\mathbb E[Z_{ie}\mid\mathcal F_G]\le0$.  Let
$E_G$ be the operational event that the raw-direction gate passes and the
subsequent e-Guard vetoes.  Then
\begin{equation}
\Pr\{E_G\mid\mathcal F_G\}
\le\sum_{e\in\mathcal E_G}\Pr\{G_e\ge100\mid\mathcal F_G\}\le.05.
\label{eq:supp-eguard-false-veto}
\end{equation}

\noindent\emph{Proof.}
For fixed $j$, every factor is nonnegative because $Z_{ie}\ge-1$ and
$j/256<1$.  The sequential path makes the product a nonnegative
supermartingale; under the independent path, factorization and AM--GM bound
its expectation by one.  Averaging preserves that bound.  Markov gives $.01$
per endpoint, and the union bound over five endpoints gives $.05$.
\hfill$\square$

The first inequality uses
$E_G\subseteq\bigcup_e\{G_e\ge100\}$; it does not condition on the
data-dependent raw-pass event.  The proposition therefore limits an
unnecessary e-Guard veto under the five pre-row conditional bounded nulls, but
does not control rejection by the raw-direction gate or give a bound after
conditioning on its pass.  It gives no bound on missed harm.  Its raw coordinate
concerns $\rho$, not the unbounded mean of $u$, and is not used in Theorem 2.

Before Certification is opened, the policy roster, incumbent, admitted action,
fixed plans, endpoint definitions, scene order, and bank identity are recorded
as immutable.  The bank is opened once and evaluated on a common paired table.
An ordinary failed component assigns the incumbent action to that policy.  A
process failure that compromises family completeness is irrecoverable unless a
separately prespecified recovery procedure can reconstruct the exact pre-Search
target; it is never silently relabeled as a statistical zero.  Reopening the
bank is prohibited, and Evaluation begins only after the terminal action for
every policy is fixed.

\begin{table}[t]
\centering
\small
\setlength{\tabcolsep}{3pt}
\begin{tabular}{p{0.29\columnwidth}p{0.63\columnwidth}}
\toprule
Terminal action & Trigger\\
\midrule
Candidate & All four fresh Certification components pass\\
Committed incumbent & Empty/capped/unresolved Search, failed raw direction,
e-Guard veto, or ordinary Certification non-release\\
Precommitted recovery target & One preauthorized Evaluation-only reconstruction
after an execution interruption, using a durable pre-Search incumbent or
structural reference; the recovery status is retained for all six policies\\
Structural scaffold & No eligible incumbent; assigned to every policy before
Search as an exact-zero intention-to-treat state\\
No analyzable terminal & The complete committed target cannot be reconstructed;
the irrecoverable cell blocks the complete 512-cell analysis and every formal claim\\
\bottomrule
\end{tabular}
\caption{Terminal semantics.}
\label{tab:terminal-states}
\end{table}

\subsection{End-to-end information boundary}

Table~\ref{tab:information-boundary} records what each stage can read and what
it must commit before the next bank opens.  This is more than an implementation
convention: Theorem~2 conditions on the entire
transcript through e-Guard, so the routed action and its plans must be immutable
before the frozen execution materializes Certification outcomes.  Evaluation
is later still and cannot alter a failed Certification decision.

\begin{table*}[t]
\centering
\small
\setlength{\tabcolsep}{4pt}
\begin{tabular}{p{0.16\textwidth}p{0.24\textwidth}p{0.27\textwidth}p{0.24\textwidth}}
\toprule
Stage & Reads & Commits before advancing & Excluded until later stage\\
\midrule
Development-B & Its disjoint Fit, Build, and direct Evaluation views &
Generator order, fallback order, and resource contracts &
All formal banks and all public-trace outcomes\\
Incumbent establishment & Formal Fit and Search/Plan view &
First verified $H_0-1$ action from the frozen generator order, including its
assignment and physical identity & Screen, Certification, and Evaluation\\
Search / Cover / Route & Search/Plan, held-out Cover, then disjoint Route rows &
Exact top-$P$, nonempty portfolio, one routed action, and fixed continuous plans &
Guard rows until routing; all Certification and Evaluation rows\\
Raw direction / e-Guard & Remaining Screen rows for the routed action only &
Forward-or-veto decision; no retry handle or portfolio access &
Certification and Evaluation\\
Certification & One fresh paired bank for the fixed action and incumbent &
Four component decisions and the terminal action & Evaluation\\
Evaluation / report & Immutable terminal actions and the common Evaluation bank &
All six policy rows, host recounts, recovery indicators, and the complete analysis &
No authority to revise an action, gate, cell roster, or hypothesis\\
\bottomrule
\end{tabular}
\caption{Data-access and commitment boundary.  ``Excluded'' indicates that the
stage does not use outcomes from that bank under the prespecified execution
order; it is an audited dependency restriction rather than a claim of physical
or cryptographic isolation.}
\label{tab:information-boundary}
\end{table*}

Ordinary rejection is represented by the committed incumbent, so it contributes
a paired zero to the intention-to-treat analysis.  An execution interruption is
different: the original bank cannot be reused, and only the prespecified
Evaluation-only procedure in Table~\ref{tab:terminal-states} may reconstruct the
incumbent or structural-target zero.  The recovery indicator is retained for
all six policies during aggregation.

\paragraph{Study-integrity note.}
Formal results are based on a single execution initiated after validation of the
analysis pipeline.  Earlier validation runs were excluded before endpoint
analysis: no endpoint estimate from them was computed, inspected, or used to
choose a method, threshold, hypothesis, or analysis rule.  Corrections were
restricted to execution safeguards and representation; the action class,
endpoints, budgets, and statistical contract were unchanged.

\section{Experimental Protocol}
\label{sec:full-protocol}

\subsection{Synthetic environment law and sample}

The confirmatory sample contains 128 i.i.d. synthetic cloud environments drawn
from the registered law $P_{\rm syn}$.  Each supplies four paired contexts:
horizons 8 and 24 crossed
with moderate and strong residual correlation.  Within a cell, roles are
disjoint: Fit 128, Build 512, Screen 512, Certification 8192, and Evaluation
512.  Build and Screen are each divided 256/256.  All methods share banks,
scene order, common random numbers, endpoint definitions, and action replays.

The population law is explicit.  For VM $i$, draw
$b_i\sim U[.15,.23]$, $a_i\sim U[.03,.09]$, a phase-group center, a normal
phase perturbation, a Rademacher loading $r_i$, and a normal scale perturbation
$z_i$.  The same environment draws are reused in its four contexts.  With
circular distance $d_H$, set
\begin{align}
p_{it}&=\exp\{-\tfrac12[d_H(t,\phi_i)/1.10]^2\},\nonumber\\
\mu_{it}&=\operatorname{clip}_{[0,.92]}(b_i+a_ip_{it}),\nonumber\\
\phi_i&=(\zeta_{g(i)}+3\epsilon_i)\bmod H,\nonumber\\
\ell_i&=(.35+.65r_i)s_i,\nonumber\\
s_i&=\operatorname{clip}_{[.35,2.5]}\{\exp(.6z_i-.18)\}.
\label{eq:synthetic-point-law}
\end{align}
For scene $s$, the common factor follows
$u_{s,t}=.55u_{s,t-1}+\sqrt{1-.55^2}\,\xi_{s,t}$.  With independent
standard-normal phase-bin shock $G$ and idiosyncratic shock $E$,
\begin{equation}
\begin{aligned}
M_{s,i,t}={}&\gamma\ell_iu_{s,t}
+\sqrt{1-.65^2}\,G_{s,\operatorname{round}(\phi_i),t}\\
&+.65E_{s,i,t}+.12\sin\{2\pi(t-\phi_i)/H\},
\end{aligned}
\label{eq:synthetic-residual-law}
\end{equation}
where $\gamma\in\{.40,.80\}$.  The realized load is
$Y_{s,i,t}=\operatorname{clip}_{[0,1.35]}
\{\mu_{it}+.045M_{s,i,t}/D_i\}$; $D_i$ is the square root of the population
random-factor variance plus sinusoid time variance, lower-bounded by $.25$.
Independent, named pseudorandom substreams determine environment, context, role,
and panel identities; outcome streams do not depend on action identifiers or
analysis results.

\begin{table*}[t]
\centering
\small
\setlength{\tabcolsep}{5pt}
\begin{tabular}{llll}
\toprule
Quantity & Value & Quantity & Value\\
\midrule
VMs / horizons & $100$ / $\{8,24\}$ & Correlation strength & $.40,.80$\\
Base / peak amplitude & $[.15,.23]$ / $[.03,.09]$ & Phase dispersion / width & $3.0/1.10$\\
Residual scale / AR(1) & $.045/.55$ & Idiosyncratic weight & $.65$\\
Scale heterogeneity & $.60$, clip $[.35,2.5]$ & Capacity / load clip & $1/[0,1.35]$\\
Fit / Build / Screen & $128/512/512$ & Certification / Evaluation & $8192/512$\\
Build / Screen split & $256+256/256+256$ & Model $z$ / shrinkage & $1.2815515655/.10$\\
$\kappa$ / tolerance & $.01/10^{-12}$ & Search $m,P$ / Cover $K$ & $8,16/4$\\
Search caps & $2{,}000{,}000$ nodes & Bound-call cap & $2{,}000{,}000$\\
\bottomrule
\end{tabular}
\caption{Registered generator, bank, and search constants.  Intervals are
population support, not method-specific tuning ranges.}
\label{tab:generator-constants}
\end{table*}

\subsection{Frozen incumbent and baseline roster}

Development-B freezes the 40-cell scale-free full-leximin winner described in
the incumbent-construction procedure above.  Its direct $H_0-1$ algorithm
action, not a release-or-$H_0$ row, is
the formal comparator construction.  Within the first nonempty generator
result, the exact projected-certificate key reranks actions and chooses
$\incp$ before \method{} Search.  The resulting comparator is therefore a
certificate-reranked frozen-generator incumbent, not a verbatim deployment of
an off-the-shelf heuristic.

\begin{table}[t]
\centering
\small
\setlength{\tabcolsep}{5pt}
\begin{tabular}{lrc}
\toprule
Generator & Eligible / 40 & Roster position\\
\midrule
Verified evacuation & 38 & 1 (selected)\\
\textsc{ProjBlind-2H} & 35 & 2\\
\textsc{Global96} & 35 & 3\\
ILS & 4 & 4\\
ALNS & 0 & 5\\
\bottomrule
\end{tabular}
\caption{Complete Development-B comparator freeze.  Eligibility is the first
selection key; full leximin of the direct-Evaluation ranks completes the frozen
rule.}
\label{tab:development-b-freeze}
\end{table}

The roster consists of:
\begin{itemize}
\item \textsc{Global96}: 96 fixed/randomized FFD orders, common covariance
feasibility, and complete replay;
\item \textsc{ProjBlind-2H}: the same incumbent-augmented problem, ordered
seeds, two-host blocks, complete action universe, $m$, $P$, and deduplication
as \method{}, but a fixed unprojected directional-mass order; the incumbent is
excluded before deduplication/top-$P$, and plans are attached relative to the
same anchor only after structural ranking;
\item verified donor evacuation with exact $H_0-1$ output; and
\item prospectively budgeted ILS and ALNS with relocate, swap, and bounded
exchange neighborhoods \cite{fleszar2002heuristics,alvim2004hybrid,
lourenco2003ils,ropke2006alns,pisinger2019lns}.
\end{itemize}
All generators obey the same capacity/covariance checks and consume the same
role-separated data.  Their method-specific node, replay, move, and wall-time
caps are fixed prospectively; we do not call unlike work units ``matched''.
Timeouts and empty sets remain visible.  The central mechanism
comparison is \method{} versus \textsc{ProjBlind-2H}, since it changes the
certificate coordinates while holding the physical search class fixed.

\subsection{Confirmatory estimand and decision rule}

Let $Y_{pcie}^{M}$ be endpoint $e$ for environment $p$, context $c$, scene
$i$, and terminal policy $M$.  For each $p$, average the paired
\method{}-minus-incumbent difference over all four contexts and Evaluation
scenes; call this cluster difference $\Delta_{pe}$.  A one-sided Student upper
endpoint $U_{.95,e}$ is formed from the 128 environment differences.  Let
$T_{pe}=\mathbf1\{\Delta_{pe}\ne0\}$ and
$B_{pe}=\mathbf1\{\Delta_{pe}<0\}$, where negative favors \method{}.  Write
$N_e=\sum_pT_{pe}$, $S_e=\sum_pT_{pe}B_{pe}$,
$n^-_e=S_e$, and $n^+_e=N_e-S_e$.  The sign $p$-value is
\begin{equation}
p^{\rm sign}_e=\Pr\{\operatorname{Bin}(N_e,1/2)\ge S_e\},
\label{eq:provider-sign-p}
\end{equation}
with value one when $N_e=0$.  Advancement requires
\begin{enumerate}
\item $U_{.95,e}<0$ and $p^{\rm sign}_e\le .05$ for every
$e\in\{J,V,R,S,\mathrm{raw}\}$; and
\item $\overline{\Delta J}\le-1/200$.
\end{enumerate}

\noindent\textbf{Proposition 4 (tie-conditional provider sign calibration).}
Condition on the full tie vector $T_e=(T_{1e},\ldots,T_{128,e})$.  If the active
signs are conditionally independent and
\begin{equation}
\Pr\{B_{pe}=1\mid T_e\}\le1/2
\quad\text{for every }p\text{ with }T_{pe}=1,
\label{eq:provider-sign-null}
\end{equation}
then Eq.~\eqref{eq:provider-sign-p} is super-uniform.  At the boundary where
every active probability is $1/2$, the conditional count has the exact
finite-sample binomial law (with the usual discreteness).  In particular, i.i.d.
draws from $P_{\rm syn}$ satisfy this premise under the provider-level null
$\Pr_{P_{\rm syn}}(\Delta_e<0\mid\Delta_e\ne0)\le1/2$.

\noindent\emph{Proof.}
Given $T_e$, couple each active $B_{pe}$ to an independent fair Bernoulli using
a common uniform.  Under Eq.~\eqref{eq:provider-sign-null}, their sum is no
larger almost surely than the fair-binomial sum, so its upper tail is
conservative.  Equality of every active success probability gives the exact
fair-binomial law. \hfill$\square$

The $J$ magnitude gate is an observed-effect safeguard, not a confidence
statement that the population effect exceeds $.005$.  The two inferential
components deliberately address different failures: the Student gate requires
a negative population mean, while the sign gate requires improvements to
outnumber worsenings among non-tied environments.  A few large gains therefore
cannot mask widespread small regressions, and many tiny gains cannot mask a
large mean regression.  Each component uses the full one-sided $.05$ level
inside one intersection--union claim; no multiplicity division is needed for
the global conjunction.  The Student statement is finite-sample exact under
i.i.d. normal cluster differences and otherwise uses the conventional
large-sample approximation for the mean.  Proposition~4 concerns the
tie-conditional probability of a negative cluster difference; it does not by
itself imply negative mean effect or an unconditional improvement probability.
Bootstrap and sign-flip summaries are sensitivities.  Both assignments are
recounted against the precommitted cell target: $H_0-1$ for an available
incumbent or $H_0$ for a structural exact-zero cell.  Thus $H$ is a structural
equality, not a statistical endpoint.

The intention-to-treat estimand includes every ordinary fallback as a zero
difference from $\incp$.  Search, no-alarm, release, and fallback rates remain
mechanism summaries.  Conditioning on released cells would answer a different,
selected question and is not used for advancement.

\section{Prospective Design Checks}
\label{sec:prospective-gates}

Two outcome-free calculations answer different design questions.  First, the
Certification sizing study fixes an action and plans that have already reached
Certification.  A preliminary $n_C=4096$ candidate did not meet the prespecified
joint lower-bound target.  For the selected $n_C=8192$, 100,000 Monte Carlo
trials gave joint four-component pass probability $.83147$, a direct 99\% lower
bound of $.82870$, and a dependence-free union lower bound of $.81480$; all
exceed $.80$.  This calculation determines only $n_C$ and excludes Search,
Route, e-Guard admission, release rate, and the environment-level primary
analysis.

\begin{table*}[t]
\centering
\small
\setlength{\tabcolsep}{4pt}
\begin{tabular}{lrrrrrl}
\toprule
Design & Trials & $J$ & $V$ & $R$ & $S$ & Joint criterion\\
\midrule
Candidate $n_C=4096$ & 10,000 & .9776 & .9249 & .9294 & .9281 &
Below target (joint bounds .7701/.7376)\\
Selected $n_C=8192$ & 100,000 & .99984 & .94015 & .94146 & .93989 &
Meets target (joint .83147; bounds .82870/.81480)\\
\bottomrule
\end{tabular}
\caption{Prospective Certification-component sizing.  ``Joint'' is the
empirical four-component pass probability for a fixed action and plans.}
\label{tab:power-gate}
\end{table*}

Second, the environment-count calculation is an outcome-free analytic
sensitivity for the 11 registered events: five zero-margin Student superiority
gates, five exact sign-dominance gates, and the $J$ observed-effect safeguard.
For the Student calculation it assumes 128 independent, approximately normal
cluster differences.  For each sign calculation it assumes
$\Pr(\Delta e<0)=.20$, $\Pr(\Delta e>0)=.02$, and tie probability $.78$.
The individual model powers are replayed exactly from the registered binary64
values below.  Applying the union bound to those 11 values, without assuming
independence among decision indicators, gives a joint lower bound of $.939247$,
above the prospective $.80$ target.

\begin{table*}[t]
\centering
\small
\setlength{\tabcolsep}{4pt}
\begin{tabular}{lrrrrrr}
\toprule
Endpoint & Model mean & Max. SD & Mean power & $p_-$ & $p_+$ & Sign power\\
\midrule
$J$ & $-.010$ & .0275440 & .992669 & .20 & .02 & .999180\\
$V$ & $-.004$ & .0110176 & .992669 & .20 & .02 & .999180\\
$R$ & $-.001$ & .00275440 & .992669 & .20 & .02 & .999180\\
$S$ & $-.010$ & .0275440 & .992669 & .20 & .02 & .999180\\
Raw & $-.00010$ & .000275440 & .992669 & .20 & .02 & .999180\\
\bottomrule
\end{tabular}
\caption{Registered $n=128$ design sensitivity for the 11 decision events.
Each endpoint contributes a zero-margin Student gate and an exact sign gate;
only $J$ adds the observed-effect safeguard.  Powers are model based, not
realized.}
\label{tab:provider-design-sensitivity}
\end{table*}

At the listed variance envelopes every Student gate has standardized effect
$.363055$ and noncentral-$t$ power $.992669$.  Each exact sign gate has power
$.999180$ under the stated three-cell model.  For $J$ alone, the safeguard
$\overline{\Delta J}\le-.005$ has standardized gap $.181527$ and normal-model
power $.98$.  No environment-power simulation was run, and this calculation
makes no claim about realized variance or achieved power.

Computational feasibility is assessed separately.  Exhaustive small instances
must agree with pruned Search under both structural-reference and explicit
incumbent anchors.  A Fit-selected stress grid records the complete unpruned
inventory, visited and pruned nodes, exact plan fits, physical replays, cap
status, wall time, and peak memory.  These measurements support implementation
feasibility; they do not alter the statistical gate or imply a runtime bound
over all cloud instances.

All registered experiments and validation checks are CPU-only on an
x86-64 Ubuntu 22.04.5 host exposing two 28-core Intel Xeon Platinum 8362
sockets (112 logical CPUs) and 935 GiB RAM.  Experiment processes pin OpenMP,
OpenBLAS, and MKL to one thread; at most three formal cells run in
parallel.  The locked environment is CPython 3.12.13 with NumPy 2.5.1, SciPy
1.18.0, pandas 3.0.3, scikit-learn 1.9.0, PyArrow 25.0.0, and matplotlib
3.11.0.  No GPU is used.

\section{Complete Results}
\label{sec:complete-results}

All result blocks are derived from the same locked analysis specification and
complete 512-cell record.  They include all 128 environments, four contexts,
five primary endpoints, structural host checks, and every fallback.  Analysis
proceeds only after verifying cell completeness, comparator and anchor identity,
and all required result fields.

\CARASuppPrimaryTable

\paragraph{Severity endpoint audit.}
$S=\min\{\mathrm{raw}/.01,1\}$ and raw severity were both retained because the
latter audits the bounded proxy used by the registered rule.  They should not
be read as empirically independent dimensions: among 262,144 Evaluation scenes
per policy, $S$ saturated in 4 scenes for \method{}, 9 for the incumbent, and
5 for \textsc{ProjBlind-2H}; the corresponding Pearson correlations between
$S$ and raw were $.999907$, $.999821$, and $.999912$.  This complete
post-outcome diagnostic leaves the registered five-endpoint analysis intact.

\subsection{Post-outcome context robustness audit}

Table~\ref{tab:context-primary-descriptive} reports the complete fixed
$4\times5$ context--endpoint roster, rather than selecting the largest
effects.  This family was constructed after outcomes were available and is
descriptive only: it cannot replace, strengthen, or reverse the registered
environment-cluster-averaged confirmatory decision.  Each of its 20 point estimates and
simultaneous one-sided upper endpoints is below zero.  This is not a claim
that every synthetic environment improved: for $J$, the four context-wise
$(n^-,n^+,n^0)$ counts are $(113,2,13)$, $(112,0,16)$, $(98,2,28)$, and
$(102,3,23)$; the continuous endpoints have no positive environment difference
but retain ties.

\begin{table*}[t]
\centering
\scriptsize
\setlength{\tabcolsep}{3.2pt}
\begin{tabular}{lrrrrr}
\toprule
Context & $J$ & $V$ & $R$ & $S$ & Raw\\
\midrule
$H=8$, moderate
& $-.04506\,[-.03439]$ & $-.02170\,[-.01780]$
& $-.003578\,[-.002936]$ & $-.01855\,[-.01531]$
& $-1.8553{\times}10^{-4}\,[-1.5310{\times}10^{-4}]$\\
$H=8$, strong
& $-.05501\,[-.04245]$ & $-.02380\,[-.01944]$
& $-.003990\,[-.003266]$ & $-.01977\,[-.01617]$
& $-1.9781{\times}10^{-4}\,[-1.6176{\times}10^{-4}]$\\
$H=24$, moderate
& $-.01656\,[-.01147]$ & $-.05782\,[-.04842]$
& $-.004145\,[-.003470]$ & $-.01806\,[-.01514]$
& $-1.8059{\times}10^{-4}\,[-1.5136{\times}10^{-4}]$\\
$H=24$, strong
& $-.02605\,[-.01858]$ & $-.06039\,[-.05004]$
& $-.004134\,[-.003432]$ & $-.01758\,[-.01459]$
& $-1.7581{\times}10^{-4}\,[-1.4585{\times}10^{-4}]$\\
\bottomrule
\end{tabular}
\caption{Complete post-outcome descriptive context audit for \method{} minus
the frozen incumbent (lower is better; 128 synthetic environment clusters and 512
Evaluation panels per cell).  Each entry is
$\widehat\Delta\,[U]$, where $U$ is the Bonferroni simultaneous one-sided
Student upper endpoint for the fixed family of 20 context--endpoint
contrasts (familywise coverage at least 95\%).  This audit cannot override
the confirmatory decision.}
\label{tab:context-primary-descriptive}
\end{table*}

\begin{figure}[t]
\centering
\CARASuppJForestPlot{}
\caption{Environment-level $\Delta J$ for \method{} minus the frozen incumbent
policy; lower is better.  Context rows use descriptive two-sided 95\% Student
intervals.  The overall row first averages the four contexts within environment
and shows the registered one-sided confidence set $(-\infty,U_{.95}]$.  Vertical
lines mark zero and the separate observed-effect safeguard $-.005$.}
\label{fig:supp-j-context-forest}
\end{figure}

\subsection{Mechanism comparisons and stage flow}

\CARASuppMechanismTable

The complete fixed-policy audit in
Table~\ref{tab:secondary-policy-descriptive} separates two findings that a
single aggregate rank would conceal.  Relative to \textsc{Global96}, ILS,
and ALNS, all 15 endpoint means and simultaneous upper endpoints favor
\method{}, and every environment-level difference is negative (128/128 for each
contrast).  The matched \textsc{ProjBlind-2H} result goes the other way:
all five point estimates are slightly positive, and none of the one-sided
simultaneous sets excludes zero in favor of \method{}.  Thus these data do
not show that certificate ordering improves terminal outcomes over the
matched structural order; no equivalence or noninferiority margin was
registered.  The entire 20-member audit is post-outcome descriptive and
cannot override the confirmatory comparison with the frozen incumbent.

\begin{table*}[t]
\centering
\scriptsize
\setlength{\tabcolsep}{0.5pt}
\resizebox{\textwidth}{!}{%
\begin{tabular}{@{}lrrrrr@{}}
\toprule
Comparator & $J$ & $V$ & $R$ & $S$ & Raw\\
\midrule
\textsc{Global96}
& $-.01416\,[-.01169]$ & $-.01065\,[-.009351]$
& $-.001252\,[-.001106]$ & $-.005891\,[-.005132]$
& $-5.8923{\times}10^{-5}\,[-5.1329{\times}10^{-5}]$\\
ILS
& $-.03286\,[-.02712]$ & $-.04018\,[-.03572]$
& $-.003838\,[-.003427]$ & $-.01781\,[-.01593]$
& $-1.7815{\times}10^{-4}\,[-1.5929{\times}10^{-4}]$\\
ALNS
& $-.03567\,[-.03007]$ & $-.04092\,[-.03645]$
& $-.003962\,[-.003553]$ & $-.01849\,[-.01662]$
& $-1.8493{\times}10^{-4}\,[-1.6623{\times}10^{-4}]$\\
\textsc{ProjBlind-2H}
& $+.000313\,[+.000942]$ & $+.000522\,[+.001215]$
& $+5.1796{\times}10^{-5}\,[+1.0728{\times}10^{-4}]$
& $+.000254\,[+.000517]$
& $+2.5405{\times}10^{-6}\,[+5.1730{\times}10^{-6}]$\\
\bottomrule
\end{tabular}}
\caption{Complete post-outcome descriptive secondary-policy audit, averaged
over the four fixed contexts (\method{} minus policy; lower is better; 128
synthetic environment clusters and 2,048 paired Evaluation panels per
environment).  Entries
are $\widehat\Delta\,[U]$ for a fixed 20-contrast Bonferroni family with
simultaneous one-sided coverage at least 95\%.  The table cannot override the
confirmatory decision.}
\label{tab:secondary-policy-descriptive}
\end{table*}

The \method{} and \textsc{ProjBlind-2H} algorithms, common action universe,
data roles, and direct paired terminal estimand were frozen before formal
outcomes.  The comparison uses the same incumbent-augmented problem, seed
inventory, eligible blocks, $m$, and $P$; it is not the difference of two
incumbent-relative summaries and does not filter unreleased cells.  No separate
mechanism superiority or equivalence gate was registered, so its statistical
contrasts are post-outcome descriptive and do not enter the advancement claim.
When
\textsc{ProjBlind-2H} is the frozen direct incumbent row, the numeric table is
retained but marked primary/direct rather than an active mechanism comparison.

Across the 512 matched cells, the two policies ended at the same physical
action in 328 cells and at different actions in 184.  Among 442 common-release
cells, 267 had the same action and 175 had different actions; three cells
released only \method{}, six released only \textsc{ProjBlind-2H}, and 61
released neither.  Table~\ref{tab:same-neighborhood-accounting} retains the
complete execution totals.  Runtime is deliberately omitted because the
stored timer scopes and provenance differ.  Nodes and bound evaluations are
also algorithm-specific counters, not comparable work units; their raw values
support auditability but no speed, cost-ratio, or efficiency claim.

\begin{table*}[t]
\centering
\scriptsize
\setlength{\tabcolsep}{4pt}
\begin{tabular}{lrrrrrr}
\toprule
Policy & Search complete & Candidates & Visited nodes & Bound evals.
& Released & Fallback\\
\midrule
\method{} & 469 & 7,504 & 32,944,186 & 28,086,939 & 445 & 67\\
\textsc{ProjBlind-2H} & 468 & 7,488 & 32,644,608 & 114,094 & 448 & 64\\
\bottomrule
\end{tabular}
\caption{Post-outcome descriptive execution accounting for the same fixed
incumbent-augmented neighborhoods (512 cells).  Candidate, node, and bound
counts are raw policy-specific audit counters; neither these counters nor the
incomparably timed runtimes support a cross-policy cost ratio.  ``Fallback''
is the committed-reference terminal.}
\label{tab:same-neighborhood-accounting}
\end{table*}

The implemented computation ablation disables pruning
while retaining exhaustive leaf ranking; its ordered top-$P$ prefix must equal
pruned Search whenever neither cap binds.  Small instances additionally use an
independent exhaustive action-universe oracle.

\subsection{Prospectively frozen shifted-Evaluation stress test}

\CARATerminalOODNarrative{}
The stress law changes only the fresh Evaluation innovations through the
registered deployment shift of $0.35$.  It preserves the 128 latent synthetic
environments and replays the two already committed terminal assignments; Fit,
Search, Guard, Certification, selection, and release are not rerun.  Thus it is
neither a new provider-population sample nor an end-to-end OOD policy test.

\CARATerminalOODPrimaryTable{}

\CARATerminalOODContextTable{}

The primary unit remains the synthetic environment after averaging its four
repeated contexts.  The complete context table is diagnostic: $J$ is tied for
all 128 environments at $H=24$ under moderate correlation, while only three
non-tied differences occur under strong correlation.  Their component failures
are retained and cannot be hidden by the environment-cluster-averaged joint pass.

\subsection{Public-trace case studies}

We treat one trace family from each of Azure, Google, and Huawei as a named
case study \cite{verma2015borg,cortez2017resourcecentral,
zhang2026cloudcons}.  Dependent windows do not create more provider labels,
so no provider-population $p$-value is reported.  Trace-specific episode
construction, block intervals, complete endpoint vectors, incumbent identity,
terminal counts, and structural host equality are shown without pooling them
with the synthetic confirmation.

The public protocol fixes four traces (Azure, two Google Borg traces, and
Huawei), 48 VMs, horizon $H=8$, and latest origin 528.  Eligible VMs have
published row length at least 536; among them, the cohort is the 48 largest
24-hour means immediately before Fit, with item identity and row index as
deterministic tie breakers.  Relative to each origin, the disjoint intervals
are Fit $[-288,-224)$, Search $[-224,-160)$, Cover $[-160,-128)$, Route
$[-128,-96)$, Guard $[-96,-64)$, short screen $[-64,0)$, and the unopened
Evaluation block $[0,8)$.  The primary analysis uses origin 528.  Origins
336, 384, 432, and 480 form an explicitly dependent, 48-hour-stride rolling
sensitivity; they are not four new providers or independent replications.

For each trace--origin cell, the frozen fallback roster selects the first
eligible $H_0-1$ action before any \method{} Search.  The record fixes the actual
generator, canonical physical action, fallback path, protocol, and structural
problem.  Search then uses an active problem that includes this incumbent when
it is not already a structural seed.  Consequently, every comparison uses a
neighborhood anchored to the actual incumbent rather than to a generator-specific
surrogate.  The tables report the generator used to construct that incumbent.

This is a shortened descriptive case-study protocol, not a second execution of
the formal experiment.  Its projected Search plans and held-out screen use
$n_C=8$ paired blocks, $P=16$, and registered node and bound-evaluation caps
of $5\times10^5$.  The frozen comparator roster remains the Development-B
roster, but a fallback cell is named by its actual generator (for example,
``ProjBlind-led frozen roster''), not presented as a pure standalone
ProjBlind run.  Neither the eight-pair screen nor its rolling sensitivity
inherits Theorem~2, a confidence statement, or provider-population scope.

\paragraph{Coverage funnel and dependence boundary.}
\CARASuppExternalNarrative

A complete post-hoc geometry audit explains all 15 empty searches.  Each
48-VM incumbent placed exactly six VMs on each of eight hosts; every two-host
union therefore contained 12 VMs and exceeded the registered $m\le8$ action
class.  The five Borg-d attempts instead contained 50--2,194 eligible blocks,
returned the full top-16, and visited 1,956--185,955 nodes.  This identifies a
fixed-neighborhood coverage boundary; it is not a post-hoc efficacy result.

\CARASuppExternalTables

\section{Integrity and Robustness Checks}
\label{sec:audit}

\paragraph{Robustness-check matrix.}
Every integrity failure is handled fail-closed: it cannot produce a nominal
candidate or statistical pass.  The matrix below summarizes the principal
perturbations and independent validation checks.
\begin{center}
\scriptsize
\setlength{\tabcolsep}{2pt}
\begin{tabular}{>{\raggedright\arraybackslash}p{0.16\columnwidth}
                >{\raggedright\arraybackslash}p{0.37\columnwidth}
                >{\raggedright\arraybackslash}p{0.37\columnwidth}}
\toprule
Boundary & Perturbation & Required response / validation\\
\midrule
Incumbent & Late selection, incorrect $H_0$ anchor, changed generator order, or
action mismatch & Reject before Search; verify temporal order, exact $H_0-1$
host count, and canonical action identity\\
Search & Non-optimistic bound, equality pruning, changed anchor, or duplicate
action & Reject on disagreement with exhaustive enumeration; compare pruning on
and off\\
Arithmetic & Near-$2^{-40}$ boundary, stale plan, or nonpositive factor & Refine
outward or reject; compare with rational and high-precision calculations\\
Data separation & Wrong role, order, count, or shared outcome storage & Reject
before use; reconstruct bank identities from the prespecified split\\
Guard / Certification & Candidate retry, changed threshold, premature access, or
bank reopening & Veto or invalidate the family; independently recompute exact
test statistics and one-use access order\\
Formal analysis & Missing row, duplicate environment, changed mean/sign gate, or
host-count substitution & Reject; independently aggregate outcomes and recount
structural assignments\\
\bottomrule
\end{tabular}
\end{center}

At each stage, inputs are treated as immutable and bound to their data role,
scene order, endpoint definitions, and action/incumbent identities.  Search
checks include zero Build differences, lattice ties, duplicate origins, an
incumbent inside the enumerated leaves, and work-cap precedence.  Statistical
checks include all-zero environment differences, constant favorable
differences, missing conditions, endpoint reordering, and exact equality at
every decision threshold.

A provenance record links the prespecified analysis, bank-opening sequence,
terminal decisions, Evaluation rows, and reported tables.  Independent
recomputation verifies one-use data access and complete policy-family
accounting.  These checks make data reuse, action substitution, and silent
omission detectable; they do not establish the scientific sampling assumptions.

\section{Additional Limitations and Deployment Notes}

The paired-sign assumption for $J$ is substantive.  A common latent shock
across Certification rows can preserve a marginal mean while invalidating the
fair-sign argument.  Likewise, the independent-average continuous proof path
cannot be combined with serial dependence, and the sequential path cannot
hide positive conditional means behind later compensation.  Immutable commitment records verify information flow, not exchangeability or
stationarity.

The study models a static homogeneous-host decision.  Migration cost, arrivals
and departures, multi-resource interference, heterogeneous hardware, priority
classes, and delayed feedback lie outside its scope.  Scenario and robust
optimization offer complementary approaches to distributional uncertainty
\cite{charnes1959chance,nemirovski2007convex,calafiore2006scenario,
campi2008exact,luedtke2008sample,pagnoncelli2009saa,campi2018general,
hadjsalem2023uncertainty,bougeret2022robust}.  Deployment would require a
prospective refresh schedule and a separate drift alarm.  The e-Guard is not
that alarm: it controls false veto under bounded no-harm nulls but offers no
false-nonveto guarantee.

Finally, $n_C=8192$ increases latency and is appropriate only when independent
replay is cheaper than an unsafe change and the incumbent is a meaningful
fallback.  The sizing calculation assumes its variance envelope; it implies
neither free samples nor frequent Guard admission.

\bibliography{references}

\end{document}
